# Supplementary material for: Spherical Inducing Features for Orthogonally-Decoupled Gaussian Processes
Source: arXiv:2304.14034 source file (2023-06-15)
Supplement: Supplementary file 1 [file rmse_summary.tex]

\begin{tabular}{lllll}
\toprule
                                       & inducing variable & \textsc{relu} features & \textsc{softplus} features & inducing points \\
                                       & kernel &                 Arccos &                     Arccos &          Arccos \\
dataset & \textsc{svgp} ($M$ inducing variables, $K$ orthogonal inducing variables) &                        &                            &                 \\
\midrule
\multirow{3}{*}{\textsc{boston} ($N=455, D=13$)} & $M=128, K=0$ &          $3.08\pm0.35$ &              $3.01\pm0.41$ &   $2.93\pm0.45$ \\
                                       & $M=128, K=128$ &          $2.48\pm0.24$ &              $2.48\pm0.24$ &   $2.85\pm0.42$ \\
                                       & $M=256, K=0$ &          $3.01\pm0.43$ &              $2.96\pm0.40$ &   $2.87\pm0.39$ \\
\cline{1-5}
\multirow{3}{*}{\textsc{naval} ($N=10740, D=14$)} & $M=128, K=0$ &          $0.01\pm0.00$ &              $0.00\pm0.00$ &   $0.00\pm0.00$ \\
                                       & $M=128, K=128$ &          $0.00\pm0.00$ &              $0.00\pm0.00$ &   $0.00\pm0.00$ \\
                                       & $M=256, K=0$ &          $0.00\pm0.00$ &              $0.00\pm0.00$ &   $0.00\pm0.00$ \\
\cline{1-5}
\multirow{3}{*}{\textsc{protein} ($N=41157, D=9$)} & $M=128, K=0$ &          $4.81\pm0.03$ &              $4.71\pm0.04$ &   $4.21\pm0.04$ \\
                                       & $M=128, K=128$ &          $4.21\pm0.05$ &              $4.20\pm0.05$ &   $4.05\pm0.04$ \\
                                       & $M=256, K=0$ &          $4.70\pm0.04$ &              $4.63\pm0.04$ &   $4.05\pm0.04$ \\
\cline{1-5}
\multirow{3}{*}{\textsc{wine (red)} ($N=1439, D=11$)} & $M=128, K=0$ &          $0.63\pm0.04$ &              $0.62\pm0.04$ &   $0.61\pm0.04$ \\
                                       & $M=128, K=128$ &          $0.62\pm0.04$ &              $0.61\pm0.04$ &   $0.61\pm0.04$ \\
                                       & $M=256, K=0$ &          $0.63\pm0.04$ &              $0.62\pm0.04$ &   $0.61\pm0.04$ \\
\cline{1-5}
\multirow{3}{*}{\textsc{wine (white)} ($N=4408, D=11$)} & $M=128, K=0$ &          $0.70\pm0.01$ &              $0.69\pm0.02$ &   $0.68\pm0.01$ \\
                                       & $M=128, K=128$ &          $0.67\pm0.01$ &              $0.67\pm0.01$ &   $0.67\pm0.01$ \\
                                       & $M=256, K=0$ &          $0.70\pm0.02$ &              $0.68\pm0.02$ &   $0.67\pm0.01$ \\
\bottomrule
\end{tabular}
